# Supplementary material for: Electrons in helical magnetic field: a new class of topological metals
Source: arXiv:2307.09884 source file (2023-07-19)
Supplement: Supplementary file 1 [file topmet_suppl.pdf]

# Supplement material to
# "Electrons in helical magnetic field: a new class of topological metals"

Yu. B. Kudasov

*Sarov Physics and Technology Institute NRNU MEPhI and*

*Russian Federal Nuclear Center - VNIIEF*

## S1. EXAMPLE FOR THEOREM 1

To illustrate theorem 1 let us consider a tight-binding model of atomic chain (nearest-neighbor hopping) with a local magnetic field corresponding to $\alpha = \pi/2$:

$$\hat{H}_{4sl} = -\sum_{i;\sigma;j=1,2,3} \left( \hat{a}^{\dagger}_{i,j,\sigma}\hat{a}_{i,j+1,\sigma} + \hat{a}^{\dagger}_{i,4,\sigma}\hat{a}_{i+1,1,\sigma} + h.c. \right) - \sum_{i,j,\sigma,\sigma'} \left( \hat{a}^{\dagger}_{i,j,\sigma}\hat{\mathbf{h}}_j\hat{a}_{i,j,\sigma'} \right). \quad \text{(S1)}$$

where $\hat{a}^{\dagger}_{i,j,\sigma}(\hat{a}_{i,j,\sigma})$ is the creation(annihilation) operator for electron in the $j$-th sublattice ($i = 1, 2, 3, 4$) and $i$-th cell with the spin projection on $z$ axis $\sigma = \pm 1/2$. A schematic representation of the chain is depicted in Fig. S1. After the Fourier transformation, we obtain the following matrix form

$$\hat{H}_k = \begin{pmatrix} 0 & h_1 & -1 & 0 & 0 & 0 & -e^{-ik} & 0 \\ h_1^* & 0 & 0 & -1 & 0 & 0 & 0 & -e^{-ik} \\ -1 & 0 & 0 & h_2 & -1 & 0 & 0 & 0 \\ 0 & -1 & h_2^* & 0 & 0 & -1 & 0 & 0 \\ 0 & 0 & -1 & 0 & 0 & h_3 & -1 & 0 \\ 0 & 0 & 0 & -1 & h_3^* & 0 & 0 & -1 \\ -e^{ik} & 0 & 0 & 0 & -1 & 0 & 0 & h_4 \\ 0 & -e^{ik} & 0 & 0 & 0 & -1 & h_4^* & 0 \end{pmatrix} \quad \text{(S2)}$$

where $h_1 = h_0$, $h_2 = -ih_0$, $h_3 = -h_0$, and $h_4 = ih_0$; $h_0$ is a real coefficient. The representation basis has the following form

$$\begin{pmatrix} 1, \uparrow \\ 1, \downarrow \\ \dots \\ 4, \uparrow \\ 4, \downarrow \end{pmatrix} \quad \text{(S3)}$$

where the first number is the sublattice number, the arrow denotes the spin state. Diagonalization of Hamiltonian (S2) gives eigenvalues shown in Fig. S1 ($h_0 = 0.4$) as dispersion curves. One can see that the dispersion curves satisfy Eq. (2). The eigenstates are at least doubly degenerate ($k \to -k$) elsewhere except the point $k = \pi$ where the degeneracy can exist (yellow circles) or do not (green circles). In the points, where the degeneracy is absent, $\langle \hat{\sigma}_z \rangle = 0$. That is why, Eq. (2) is fulfilled for the nondegenerate states also. There is an additional degeneracy at $E = 0$.

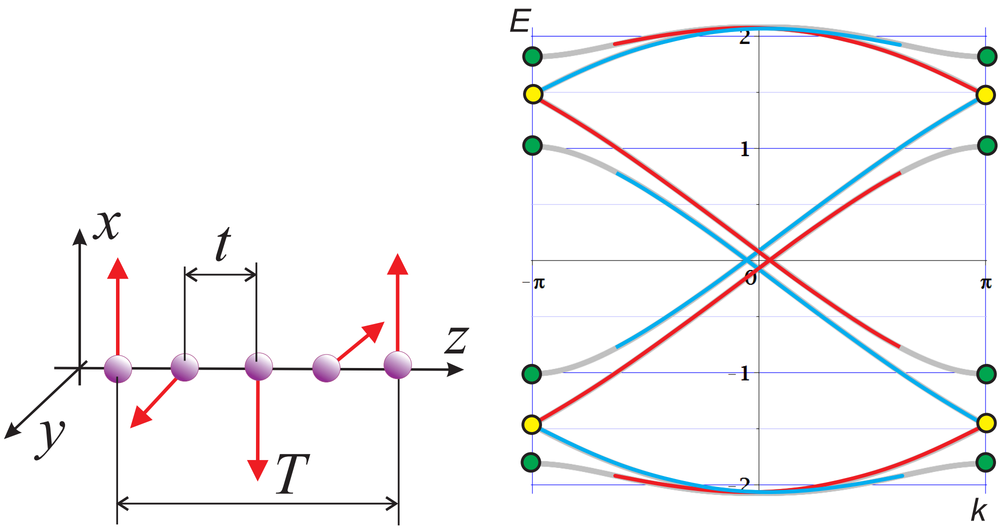


FIG. S1. The 1D tight-binding model for four-sublattice helical model ($\alpha = \pi/2$): a schematic view (left panel) and the electron dispersion (right panel). The arrows show directions of $\hat{\mathbf{h}}_j$. The average spin along the dispersion curves is indicated by color: red and blue if $|\langle\hat{\sigma}_z\rangle| > 1/2$, gray otherwise. The yellow and green circles denote the degenerate and non-degenerate points, correspondingly.

## S2. ON THEOREM 2

The relations for transverse spin components $\langle\hat{\sigma}_{x(y)}\rangle_{\mathbf{k}} = 0$ can be proven by direct calculations. The average of spin projection on $x$ axis is defined by

$$S_x = \frac{1}{V}\int_V \varphi^*_{\mathbf{k}}(\mathbf{r})\hat{\sigma}_x\varphi_{\mathbf{k}}(\mathbf{r})d\mathbf{r} \tag{S4}$$

where the integration is performed over the magnetic unit cell and $V$ is its volume. However, there are alternative choices of the magnetic unit cell, e.g. one can shift it by generalized translations by $\hat{\mathbf{t}\mathbf{r}}_\alpha$ or $\hat{-\mathbf{t}\mathbf{r}}_{-\alpha}$. The only effect of these operations is the spin rotation about $z$ axis:

$$\begin{aligned} S'_x &= \cos(\alpha)S_x + \sin(\alpha)S_y \\ S''_x &= \cos(\alpha)S_x - \sin(\alpha)S_y. \end{aligned} \tag{S5}$$

Since the average of spin projection should be independent on the particular choice of the cell, $S_x = S'_x = S''_x$. It is easy to see that the only solution of the equations is $S_x = 0$ (apart from the trivial solution $\cos(\alpha) = 1$). The identity $S_y = 0$ can be proved similarly.

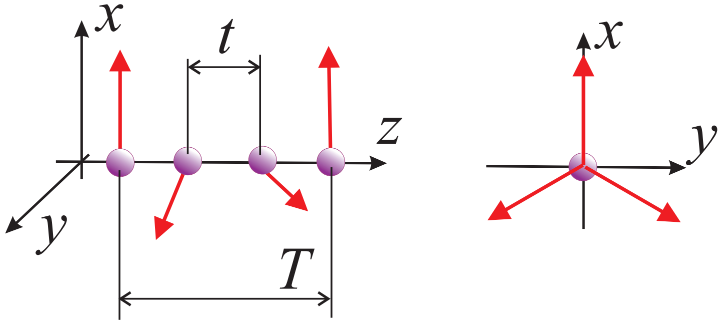


FIG. S2. A schematic view of the three-sublattice 1D chain as an illustration of the tight-binding model ($\alpha = 2\pi/3$) Eq. (10).

## S3. EXAMPLE FOR THEOREM 2

A schematic representation of the three-sublattice tight-binding model with $120^0$ helical effective field Eq. (10) is shown in Fig. S2. After the Fourier transformation, the model is reduced to the following matrix form

$$\hat{H}_k = \begin{pmatrix} 0 & h_1 & -1 & 0 & -e^{-ik} & 0 \\ h_1^* & 0 & 0 & -1 & 0 & -e^{-ik} \\ -1 & 0 & 0 & h_2 & -1 & 0 \\ 0 & -1 & h_2^* & 0 & 0 & -1 \\ -e^{ik} & 0 & -1 & 0 & 0 & h_3 \\ 0 & -e^{ik} & 0 & -1 & h_3^* & 0 \end{pmatrix} \tag{S6}$$

where $h_1 = h_0$, $h_2 = h_0(-1 - i\sqrt{3})/2$, and $h_3 = h_0(-1 + i\sqrt{3})/2$. A result of Hamiltonian diagonalization for $h_0 = 0.2$ is shown in Fig. 1.

## S4. 2D NEARLY-FREE-ELECTRON MODEL

A 2D nearly-free-electron model should contain at least two terms in the sum in Eq. (11) because two Bragg planes intersect at K points of the Brillouin zone as shown in Fig. S3. This is the minimal 2D nearly-free-electron model which was used.

A model effective field corresponding to the $120^0$ helical magnetic field has the following

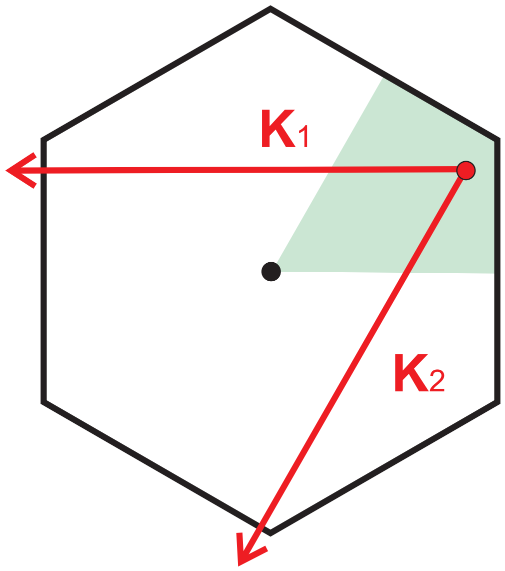


FIG. S3. The 2D magnetic Brillouin zone and its irreducible part (fill area). A pair of vectors of reciprocal lattice, which are taken into account in the sum in Eq. (11), are shown by red color.

form

$$h_x = \cos(\mathbf{K}_1\mathbf{r}) + \sin(\mathbf{K}_2\mathbf{r}) + \cos(\mathbf{K}_3\mathbf{r}),$$
$$h_y = \sin(\mathbf{K}_1\mathbf{r}) + \cos(\mathbf{K}_2\mathbf{r}) + \sin(\mathbf{K}_3\mathbf{r}) \tag{S7}$$

where $\mathbf{K}_i$ are the vectors of magnetic reciprocal lattice. A distribution of the effective magnetic field is shown in Fig. S4. The Fourier coefficients are $\hat{U}_{\mathbf{K}_{1(2)}} = h_0\big(\hat{\sigma}_x \pm i\hat{\sigma}_y\big)/2$. The coefficients do not depend on the specific form of the magnetic potential up to a complex constant [21]. These spinor Fourier coefficients are abnormal operators, i.e. $\hat{U}_{\mathbf{K}}\hat{U}^{\dagger}_{\mathbf{K}} \neq \hat{U}^{\dagger}_{\mathbf{K}}\hat{U}_{\mathbf{K}}$. That is why, $\hat{U}_{\mathbf{K}}\hat{U}_{-\mathbf{K}} \neq \hat{U}_{-\mathbf{K}}\hat{U}_{\mathbf{K}}$ that leads to unusual properties against time reversion in the nearly-free-electron model [21].

The dispersion of 2D model is shown in Fig. S5. Three sheets of the dispersion surface are periodic as a whole to satisfy the Bloch theorem $(E_{l,\mathbf{k}+\mathbf{K}} = E_{l,\mathbf{k}})$ . At the same time, an isolated sheet is non-periodic, i.e. while a sheet crosses a border of the magnetic Brillouin zone it changes the eigenvalue number $l$ (see Fig.S5). One can also see that the sheets crossing occurs at the magnetic Brillouin zone boundaries and along the Γ-K line.

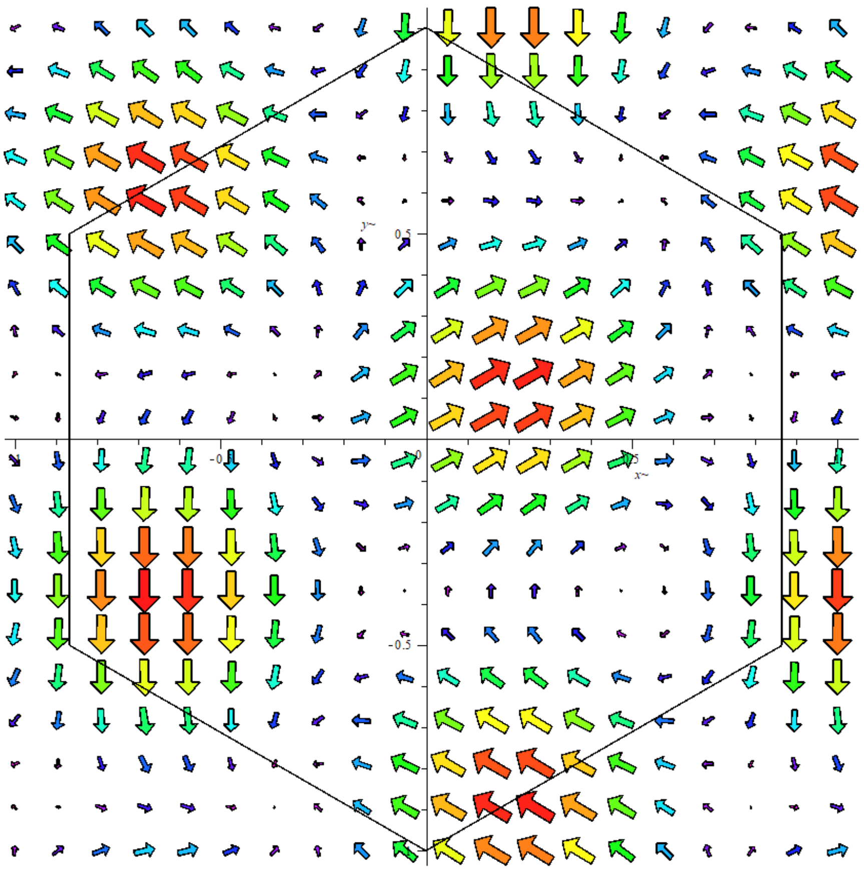

FIG. S4. A schematic view of the model $120^0$ effective field distribution Eq.(S7). The magnetic unit cell is shown by hexagon.

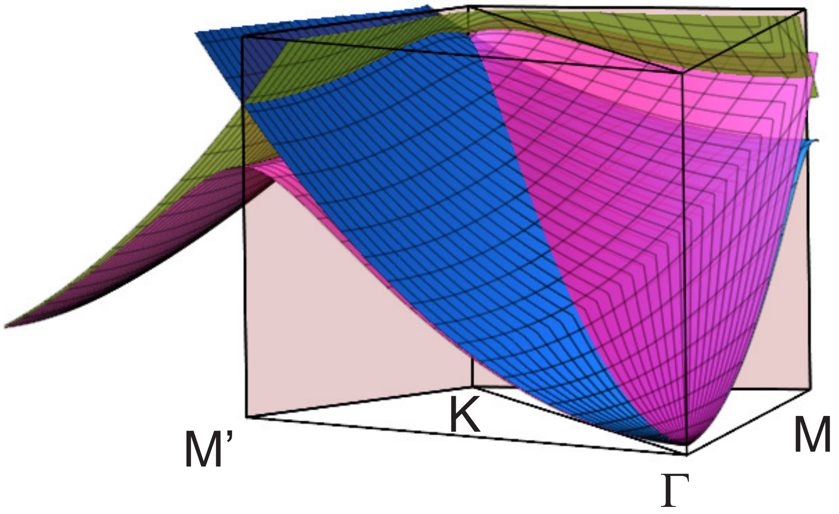


FIG. S5. The three lowest dispersion sheets (shown by color) and irreducible part of the magnetic Brillouin zone.
